# Supplementary material for: Exploring Self-attention for Image Recognition
Source: arXiv:2004.13621 source file (2020-04-28)
Supplement: Supplementary file 1 [file supplement.tex]

\section{Network Architecture}
\label{sec:architecture}

\newcommand{\blockres}[3]{\multirow{3}{*}{
		\(\left[
		\begin{array}{l}
		\text{linear, 1$\times$1, #2}\\
		[-.1em] \text{conv, 3$\times$3, #2}\\
		[-.1em] \text{linear, 1$\times$1, #1}
		\end{array}\right]\)$\times$#3}
}

\newcommand{\blocksan}[3]{\multirow{3}{*}{
		\(\left[
		\begin{array}{l}
		\text{linear, 1$\times$1, #2}\\
		[-.1em] \text{sab, 3$\times$3, #2}\\
		[-.1em] \text{linear, 1$\times$1, #1}\\
		\end{array}\right]\)$\times$#3}
}

\newcommand{\blocksanx}[3]{\multirow{3}{*}{
		\(\left[
		\begin{array}{l}
		\text{linear, 1$\times$1, #2}\\
		[-.1em] \text{sab, 3$\times$3, #2, $C$=32}\\
		[-.1em] \text{linear, 1$\times$1, #1}\\
		\end{array}\right]\)$\times$#3}
}
\newcolumntype{x}[1]{>\centering p{#1pt}}
\begin{table}[t]
\footnotesize
\begin{center}
{\scalebox{0.95}{
\begin{tabular}{c|c}
\hline
output & SAN-50 \\
\hline
112$\times$112 & conv, $7\times7$, $64$, stride $2$ \\
\hline
\multirow{4}{*}{56$\times$56} & max pool, $3\times3$, stride $2$ \\
& \blocksan{256}{64}{3} \\
& \\
& \\
\hline
\multirow{3}{*}{28$\times$28} & \blocksan{512}{128}{4} \\
& \\
& \\
\hline
\multirow{3}{*}{14$\times$14} & \blocksan{1024}{256}{6} \\
& \\
& \\
\hline
\multirow{3}{*}{7$\times$7} & \blocksan{2048}{512}{3} \\
& \\
& \\
\hline
$1\times1$ & global average pool, $1000$-d $fc$, softmax \\
\hline
\end{tabular}}}
\end{center}
\caption{\small Architectures of self-attention networks based on ResNet for ImageNet classification.}
\label{tab:arch}
\end{table}
